# Supplementary material for: TANDEM: Balancing Centralized and Decentralized Critics to Address the Information Gap in Complex Multi-Agent Environments
Source: arXiv:2610.37592 source file (2026-10-27)
Supplement: Supplementary file 1 [file supplementary.tex]

\documentclass[sigconf,anonymous]{aamas}

\usepackage{amsmath}
\usepackage{graphicx}
\usepackage{booktabs}
\usepackage{makecell}
\microtypesetup{expansion=false}
% Number supplement tables/figures as S1, S2, ... so the main paper's "Table S1"
% references match.
\renewcommand{\thetable}{S\arabic{table}}
\renewcommand{\thefigure}{S\arabic{figure}}

%%% AAMAS-2027 copyright block (do not change).
\makeatletter
\gdef\@copyrightpermission{
  \begin{minipage}{0.2\columnwidth}
   \href{https://creativecommons.org/licenses/by/4.0/}{\includegraphics[width=0.90\textwidth]{by}}
  \end{minipage}\hfill
  \begin{minipage}{0.8\columnwidth}
   \href{https://creativecommons.org/licenses/by/4.0/}{This work is licensed under a Creative Commons Attribution International 4.0 License.}
  \end{minipage}
  \vspace{5pt}
}
\makeatother
\setcopyright{ifaamas}
\acmConference[AAMAS 2027]{Proc.\@ of the 26th International Conference
on Autonomous Agents and Multiagent Systems (AAMAS 2027)}{3--7 May 2027}{Hanoi, Vietnam}{M.~Baldoni, F.~Fang, W.~Yeoh, N.~Yorke-Smith (eds.)}
\copyrightyear{2027}
\acmYear{2027}
\acmDOI{}
\acmISBN{}

\title{Supplementary Material\\ TANDEM: Balancing Centralized and Decentralized
Critics to Address the Information Gap in Complex Multi-Agent Environments}

\author{Anonymous Author(s)}
\affiliation{%
  \institution{Submission under double-blind review}
  \city{}
  \country{}}
\email{}

\begin{document}
\maketitle

\renewcommand{\thetable}{S\arabic{table}}

\input{sections/11-supplementary}

\end{document}
